# Supplementary material for: A framework for implementing general virtual element spaces
Source: arXiv:2208.08978 source file (2023-11-20)
Supplement: Supplementary file 1 [file appendix.tex]

\appendix
\label{sec: appendix}
\section{Laplace}\label{appendix: laplace}
\lstinputlisting[language=python]{mixed/laplace.py}
\section{Navier-Stokes}\label{appendix: navier stokes}
\lstinputlisting[language=python]{navierStokes/cylinderUzawa.py}
\section{Willmore flow}\label{appendix: willmore}
\lstinputlisting[language=python]{willmore/willmore.py}
